# Supplementary material for: Double-mode relaxation of highly deformed vesicles
Source: arXiv:2003.02063 source file (2020-02-27)
Supplement: Supplementary file 1 [file SI.pdf]

# Supporting Information: Double-mode relaxation of highly deformed vesicles

Dinesh Kumar,[1,2] Channing M. Richter,[1] and Charles M. Schroeder[1,2,3,*]

[1]*Department of Chemical and Biomolecular Engineering University of Illinois at Urbana-Champaign, Urbana, IL, 61801*
[2]*Beckman Institute for Advanced Science and Technology University of Illinois at Urbana-Champaign, Urbana, IL, 61801*
[3]*Department of Materials Science and Engineering University of Illinois at Urbana-Champaign, Urbana, IL, 61801*

(Dated: February 27, 2020)

## Supplementary Text

### Vesicle preparation

Giant unilamellar vesicles (GUVs) are prepared from a mixture of 1,2-dioleoyl-sn-glycero-3-phosphocholine (DOPC, Avanti Polar Lipids) and 0.12 mol % of the fluorescent 1,2-dioleoyl-sn-glycero-3-phosphoethanolamine-N-(lissamine rhodamine B sulfonyl (DOPE-Rh, ex/em 560nm/583nm, Avanti Polar Lipids) for visualization purposes by using the standard electroformation method described by Angelova *et al.* [1]. In our work, the fluorescent lipid contains the fluorescent dye (Rhodamine) on the lipid head group (rather than the tail group) because it is known that lipids with labeled hydrocarbon tails (e.g. NBD-PC) could result in perturbed membranes because the charged dye molecule tends to 'flip up' into the head group space, which can affect the bending modulus of the lipid membrane [2].

For electroformation, a stock lipid solution is made with 25 mg/mL DOPC and 0.04 mg/mL DOPE-Rh. Next, 10 $\mu$L of the lipid solution in chloroform is spread on a conductive indium tin oxide (ITO) coated glass slide (resistance $\approx$ 35 $\Omega$, 25 $\times$ 50 $\times$ 1.1 mm, Delta Technologies) and dried under vacuum overnight for solvent drying. A 1.5 mm Teflon spacer is sandwiched between the pair of ITO slides, thereby forming a chamber with $\approx$ 2.4 mL of volume and coupled to a function generator (Agilent 33220 A). The electroformation chamber is filled with 100 mM sucrose solution (Sigma-Aldrich) and an AC electric field of 2 V/mm at 10 Hz is applied for 120 min at room temperature (22°C). At room temperature, DOPC lipid remains in the fluid phase. Most of the vesicles prepared by this method are unilamellar with few defects and in the size range of 5 to 30 $\mu$m in radius. Multilamellar vesicles are not considered or analyzed for these experiments.

The viscosity of 100 mM sucrose solution ($\mu$ = 1.1 mPa·s) is measured using a benchtop viscometer (Brookfield) at 22°C. Most of the vesicles obtained after electroformation are quasi-spherical in nature. To generate deflated (low reduced volume) vesicles, a small amount of 200 mM sucrose solution is added to the vesicle suspension, which drives water out of the vesicle interior to until the sucrose concentrations are equal on both sides of the membrane [2, 3]. This protocol of osmotic deflation produced low reduced volume vesicles in the range $0.20 < \nu < 0.80$. However, the overall number of very low reduced volume vesicles in the suspension is generally small.

### Experimental setup

Single-layer microfluidic devices (width = 400 $\mu$m, and depth = 100 $\mu$m) are fabricated using standard soft lithography techniques [4]. In brief, a thin layer ($\approx$ 100 $\mu$m) of negative photoresist (SU8 2050) was transferred to a 3" diameter silicon wafer using spin coating. Next, the microfluidic channels were patterned on the photoresist using UV exposure through a high quality transparency mask (CAD/Art Services Inc.). The exposed photoresist was then developed in propylene glycol monomethyl ether acetate (PGMEA) to yield a mold. The mold was then treated with trichloro (1H, 1H, 2H, 2H-perfluorooctyl) silane vapor to enable facile removal of the polydimethylsiloxane (PDMS) device after replica molding. PDMS was prepared using a 10:1 (w/w) base:crosslinker ratio and poured onto the mold in a careful manner to prevent the formation of bubbles, followed by overnight baking at 65 $^o$C. The slab of PDMS containing the microfluidic device was then cut out using a razor blade and holes for the inlet channels were punched using a needle with a blunt tip. This device was then bonded to a glass coverslip using plasma oxidation to yield the final device.

A schematic of the experimental set up is shown in Fig. S1. Microfluidic devices are mounted on an inverted fluorescence microscope (Olympus IX71), which allows for real-time imaging of fluorescent vesicles using a 10x mag-

nification air-immersion objective lens and a 100-W mercury arc lamp (USH102D, UShio). The sucrose buffer is introduced into microfluidic devices using four pressure regulators (MPV series, Proportion Air) which are actuated through a computer controlled LabVIEW data acquisition device with analog input and output capabilities (NI 9264, NI9205 and NI9174, National Instruments). Each output pressure line from the regulators is connected to a fluidic reservoir containing the sample (Elveflow XS fluid reservoir), which is connected to the microfluidic device using FEP and PEEK tubing (IDEX Health and Science). Tube dimensions (inner diameter and length) are chosen such the fluidic resistance within the tubing is significantly larger than the fluidic resistance of the microfluidic channels. Vesicles are imaged using a CCD camera (GS3-U3-120S6M-C, 1920 $\times$ 1200 pixels, 30 fps) with a pixel size is 0.586 $\mu$m. Experimental trajectories were analyzed using custom MATLAB codes.

### Relaxation of quasi-spherical vesicles

For the quasi-spherical vesicle shown in Fig. S2 and Fig. S3, the fast retraction of vesicle shape occurs within approximately 500 ms, which is $\approx$15 $\times$ larger than the inverse sampling rate of the CCD camera (33 ms). These results suggest that quasi-spherical vesicles exhibit a fast relaxation process, though the precise determination of these timescales for quasi-spherical vesicles would require sampling vesicle relaxation dynamics at a faster rate (e.g. using a CCD camera with larger sampling rate). In this manuscript, our results mainly focus on the relaxation of slightly deflated vesicles, with characteristic relaxation timescales much longer than the integration time of the CCD camera. Nevertheless, quasi-spherical vesicles have been widely studied in the literature [5, 6] and our observations are generally consistent with prior work. The slower relaxation time scale $\tau_2 = 5$ s obtained by a single exponential fit (Fig. S3) is on the order of $\tau_2 = \mu L_{trans}/\sigma_0$, consistent with the data for vesicles with $\nu < 0.75$ presented in the main text.

### Bending and area stretching regimes of vesicles

Vesicle deformation can occur in two different regimes: (i) the bending deformation regime, wherein the membrane undulations due to thermal fluctuations of non-spherical vesicles with large surface area-to-volume ratios are gradually smoothened out, and (ii) the stretching deformation regime, wherein membrane stretching occurs and the total area of bilayer membrane increases. In this work, our results focus solely on vesicle stretching in the bending-dominated regime. In this regime, the membrane tension increases exponentially with the change in projected area [7].

During vesicle stretching, the increase in projected area due to contributions from smoothing out thermal fluctuations and area stretching is given as:

$$\frac{A - A_0}{A_0} = \frac{k_B T}{8\pi\kappa} ln\left(\frac{\sigma}{\sigma_0}\right) + \frac{\sigma}{K_a} \tag{S1}$$

where $A_0$ is the initial in-plane area, $A$ is the projected area at a given time during the deformation step, $\kappa$ is the bending modulus, $k_B$ is the Boltzmann constant, $T$ is the temperature, $\sigma$ is the membrane tension during the deformation, $\sigma_0$ is the initial tension, and $K_a$ is the area stretching modulus. The cross-over from the bending to stretching regime occurs when the contribution from two terms in Eq. (S1) becomes equal. This leads to the cross-over tension $\sigma_c = K_a k_B T/8\pi\kappa$. For typical values of the parameters for a lipid vesicle namely $K_a = 0.1$ N/m, $\kappa = 25 k_B T$, the cross-over tension $\sigma_c \approx 0.1$ mN/m.

For flow stretching experiments, the tension induced on the vesicle membrane during the deformation step is related to the fluid strain-rate of the externally imposed flow. Following the approach in [8], we can estimate the maximum tension in the tether as a function of fluid strain-rate:

$$\sigma_{max} \approx \frac{\mu^2 \dot{\epsilon}^2 R^4}{\kappa} \tag{S2}$$

For our experiments, the typical parameters used in this work are $\mu = 0.0011$ Pa-s, $\dot{\epsilon} = 5\ s^{-1}$, $R$ =10 $\mu$m. Based on our experimental conditions, the maximum tension induced in the membrane is $\sigma_{max} = 0.02$ mN/m, which is more than one order of magnitude smaller than the cross-over tension for area stretching. The values of maximum tension induced in each vesicle in this work is included in the Table S1. Evidently, the contribution from area stretching is negligible for the parametric ranges considered in this work.

### Effect of deformation strain-rate on relaxation trajectories

In Fig. S7, two representative vesicles are shown with reduced volumes $\nu = 0.43$ and 0.72. These vesicles are stretched several times at different strain-rates. Upon increasing the fluid strain-rate, the vesicle undergoes higher aspect ratio $L/L_0 - 1$ deformation. However, the fast time-scale $\tau_1$ approximately remains same in the range of strain-rates used in our experiments, as shown in Table S2.

### Characterization of slow relaxation time scale, $\tau_2$

Prior to the beginning of slow relaxation phase, most of the bending energy stored in the thin tether has been released. For this reason, we assume that the membrane tension is constant during the slow relaxation phase. The numerical values of the slow double-mode time scale $\tau_2$ are on the order of tension time-scale $t_{surf} = \mu L_{trans}/\sigma_0$ as shown in Fig. S8. Here, $L_{trans}$ is the vesicle stretch along the extensional axis at the beginning of slow retraction step and $\sigma_0$ is the ensemble-averaged membrane tension.

Due to the nature of electroformation method [2, 9, 10], the membrane tension $\sigma_0$ for each vesicle in the ensemble is different and generally varies based on the degree of osmotic deflation. In prior work [10], we estimated the ensemble-averaged membrane tension for quasi-spherical shapes to be $\approx 10^{-8}$ N/m, which is used to scale $\tau_2$. We typically observe that this value of $\sigma_0$ can vary by at least one order of magnitude (larger or smaller), as electroformation method does not generate vesicles with well-defined tensions. Due to these complexities, we use the ensemble-averaged value for $\sigma_0$ in the scaling argument. Nevertheless, the numerical values of normalized slow double-mode time are on the order of tension time-scale for all the vesicles in our experiments, at least within a factor of ≈5-10. We note that the slow relaxation time can vary from 20 seconds to minutes depending on the extent of the deformed aspect ratio of the vesicle.

Taken together, our results suggest that the slow relaxation phase of vesicles (governed by membrane tension-driven relaxation processes) is analogous to the relaxation of highly deformed dumbbell-shaped Newtonian fluid drops, whose relaxation time scaling has been established as $\mu L/\sigma$ in prior work using computer controlled four-roll mill [11]. Here, $\mu$ is the viscosity of suspending medium, $L$ is the length of drop at the beginning of relaxation phase, and $\sigma$ is the surface tension of drop fluid and suspending fluid interface.

### Viscoelastic model for vesicle relaxation

In the main text, a linear viscoelastic model is used to represent the double mode exponential relaxation of vesicle membrane. In this model, the stress can be divided into sum of two terms:

$$\sigma = \sigma_1 + \sigma_2 \tag{S3}$$

where $\sigma_1$ is the stress in left Maxwell-element and $\sigma_2$ in the right element as shown in Fig. 3 in the main text. The stress-relaxation constitutive model can be written as [12]:

$$\frac{\sigma}{\eta_1\eta_2} + \left(\frac{1}{\eta_1 E_2} + \frac{1}{\eta_1 E_1}\right)\frac{\mathrm{d}\sigma}{\mathrm{d}t} + \frac{1}{E_1 E_2}\frac{\mathrm{d}^2\sigma}{\mathrm{d}t^2} = \left(\frac{1}{\eta_1} + \frac{1}{\eta_2}\right)\frac{\mathrm{d}\varepsilon}{\mathrm{d}t} + \left(\frac{1}{E_1} + \frac{1}{E_2}\right)\frac{\mathrm{d}^2\varepsilon}{\mathrm{d}t^2} \tag{S4}$$

where $\eta_1, \eta_2$ are the viscosities of the dashpots, $E_1, E_2$ are the spring constants, and $\varepsilon$ is the strain in the material.

Here, we consider the particular case of stress-relaxation. The initial condition and the boundary condition are:

$$\sigma = 0 \; at \; t = 0, \tag{S5}$$

$$\varepsilon(t) = \varepsilon_0 H(t)) \tag{S6}$$

where $H(t)$ is the Heaviside function and $\varepsilon_0$ is the strain on the material at $t = 0$.

Other useful mathematical definitions used in deriving the model are:

$$\frac{\mathrm{d}H(t))}{\mathrm{d}t} = \delta(t) \tag{S7}$$

$$\mathcal{L}\left(\frac{\mathrm{d}^2 H(t))}{\mathrm{d}t^2}\right) = S \tag{S8}$$

$$\mathcal{L}\left(\sigma(t)\right) = Y \tag{S9}$$

$$\dot{\sigma}(0^+) = 0 \tag{S10}$$

$$\dot{\sigma}(0^-) \neq 0 \tag{S11}$$

where $\mathcal{L}$ is the Laplace transform of a function.

Taking Laplace transform on both sides of Eq. (S4),

$$Y + \left(\frac{\eta_2}{E_2} + \frac{\eta_1}{E_1}\right) SY + \frac{\eta_1\eta_2}{E_1E_2}\mathcal{S}^2 Y = (\eta_1 + \eta_2)\varepsilon_0 + \mathcal{S}\varepsilon_0\left(\frac{\eta_1\eta_2}{E_1} + \frac{\eta_1\eta_2}{E_2}\right) \tag{S12}$$

$$Y = \varepsilon_0 \frac{\eta_1\eta_2 + \left(\frac{\eta_1\eta_2}{E_1} + \frac{\eta_1\eta_2}{E_2}\right)\mathcal{S}}{1 + S\left(\frac{\eta_2}{E_2} + \frac{\eta_1}{E_1}\right) + S^2\frac{\eta_1\eta_2}{E_1E_2}} \tag{S13}$$

Taking the inverse Laplace transform on both sides, we obtain the stress-relaxation as:

$$\sigma(t) = \varepsilon_0\left[E_1 e^{\frac{-t}{\eta_1/E_1}} + E_2 e^{\frac{-t}{\eta_2/E_2}}\right] \tag{S14}$$

The stress-relaxation modulus of the material following Eq. (S14) is written as:

$$G(t) = E_1 e^{\frac{-t}{\eta_1/E_1}} + E_2 e^{\frac{-t}{\eta_2/E_2}} \tag{S15}$$

Finally, the storage and loss modulus can be written as:

$$G'(\omega) = \omega\int_0^\infty dt\sin(\omega t)G(t)dt \tag{S16}$$

$$G''(\omega) = \omega\int_0^\infty dt\cos(\omega t)G(t)dt \tag{S17}$$

$$G'(\omega) = \frac{E_1\left(\omega\frac{\eta_1}{E_1}\right)^2}{1 + \left(\omega\frac{\eta_1}{E_1}\right)^2} + \frac{E_2\left(\omega\frac{\eta_2}{E_2}\right)^2}{1 + \left(\omega\frac{\eta_2}{E_2}\right)^2} \tag{S18}$$

$$G''(\omega) = \frac{E_1\omega\frac{\eta_1}{E_1}}{1 + \left(\omega\frac{\eta_1}{E_1}\right)^2} + \frac{E_2\omega\frac{\eta_2}{E_2}}{1 + \left(\omega\frac{\eta_2}{E_2}\right)^2} \tag{S19}$$

The stress $\sigma(t)$ and initial strain $\varepsilon_0$ in Eq. (S14) can be expressed as:

$$\sigma(t) = F(t)/A_0 \tag{S20}$$

$$\varepsilon_0 = \frac{L_{max} - L_0}{L_0} \tag{S21}$$

Here, $F(t)$ is the force, $A_0$ is the area of vesicle, and $L_0$ is the initial vesicle length along the axis of extension at the

beginning of deformation. We approximate the force $F(t) \approx 6\pi\mu R_{v1}\frac{dL}{dt}$ and the area $A_0 = 4\pi R_{v1}^2 + 4\pi R_{v2}^2 + 2\pi R_t L_t$ where $R_{v1}$ is the radius of spherical bulb eating the tether, $R_{v2}$ is the radius of other spherical end at the beginning of relaxation, $R_t$ is the thin tether radius and $L_t$ is tube length at the start of relaxation. The tether radius $R_t$ is estimated as $\kappa/3\mu\dot{\epsilon}R_{v1}^2$ [8]. Eq. (S14) is simplified to:

$$6\pi\mu R_{v1} dL = A_0(L_{max} - L_0)/L_0 \left[E_1 e^{-t/\left(\frac{\eta_1}{E_1}\right)} + E_2 e^{-t/\left(\frac{\eta_2}{E_2}\right)}\right] dt \tag{S22}$$

Integrating both sides, the final expression for time-dependent vesicle length $L(t)$ becomes:

$$L(t) = L_{max} - B'\left(1 - e^{-t/\left(\frac{\eta_1}{E_1}\right)}\right) - C'\left(1 - e^{-t/\left(\frac{\eta_2}{E_2}\right)}\right) \tag{S23}$$

Finally, we write an approximate model for the vesicle aspect ratio during relaxation as follows:

$$L(t)/L_0 - 1 = A' + B' e^{-t/\left(\frac{\eta_1}{E_1}\right)} + C' e^{-t/\left(\frac{\eta_2}{E_2}\right)} \tag{S24}$$

Here, the parameters $A'$, $B'$ and $C'$ are expressed in terms of the known quantities as:

$$A' = \frac{L_{max}}{L_0} - 1 - B' - C' \tag{S25}$$

$$B' = \frac{A_0}{6\pi\mu R_{v1}} \frac{L_{max} - L_0}{L_0} \eta_1 \tag{S26}$$

$$C' = \frac{A_0}{6\pi\mu R_{v1}} \frac{L_{max} - L_0}{L_0} \eta_2 \tag{S27}$$

Eq. (S24) is fit to the vesicle relaxation trajectories, and the viscoelastic model parameters $\eta_1, \eta_2$ and $E_1, E_2$ are estimated.

# Supplementary Tables

| $\nu$ | $\dot{\epsilon}$ $(s^{-1})$ | $\tau_1$ $(s)$ | $\tau_2$ $(s)$ | $R^2$ value | $R$ $(\mu m)$ | $\sigma_{max}$ $(\mu N/m)$ | $t_{bend}$ | $t_{surf}$ |
|---|---|---|---|---|---|---|---|---|
| 0.74 | 7.40 | 2.1 | 16.04 | 0.9896 | 10.4 | 19 | 13.5 | 6.6 |
| 0.72 | 5.88 | 8.64 | 112.14 | 0.9972 | 12.5 | 25 | 23.4 | 7.8 |
| 0.70 | 2.44 | 5 | 197.7 | 0.9903 | 9.9 | 1.8 | 11.9 | 11.7 |
| 0.67 | 3.42 | 0.87 | 16.53 | 0.9705 | 6.2 | 0.50 | 2.9 | 4.6 |
| 0.59 | 9.98 | 0.77 | 60.4 | 0.9593 | 5.2 | 2.1 | 1.6 | 7.0 |
| 0.55 | 3.54 | 10.1 | 639 | 0.9748 | 14.6 | 17 | 37.3 | 41.8 |
| 0.50 | 3.40 | 4.2 | 32 | 0.9729 | 4.8 | 18 | 12.2 | 7.3 |
| 0.43 | 0.61 | 5.74 | 152.67 | 0.9953 | 8.6 | 0.6 | 7.6 | 14.5 |
| 0.40 | 0.83 | 4.27 | 29.2 | 0.9965 | 7.8 | 0.08 | 5.8 | 30.2 |
| 0.37 | 0.83 | 3.14 | 114.32 | 0.9865 | 6.5 | 0.04 | 3.3 | 15.8 |
| 0.25 | 2.15 | 6.9 | 113.41 | 0.9907 | 8.4 | 0.70 | 7.1 | 35.9 |

TABLE S1. Experimental parameters for non-spherical vesicles as shown in Fig. 2 in the main text.

| $\nu$ | $\tau_1$ $(s)$ | $\tau_2$ $(s)$ |
|---|---|---|
| 0.43 | 5.70 | 108.24 |
| 0.43 | 5.64 | 118.34 |
| 0.43 | 5.74 | 152.67 |
| 0.72 | 8.66 | 88.67 |
| 0.72 | 8.64 | 112.14 |

TABLE S2. Experimental parameters for the vesicles shown in Fig. S7.

# Supplementary Figures

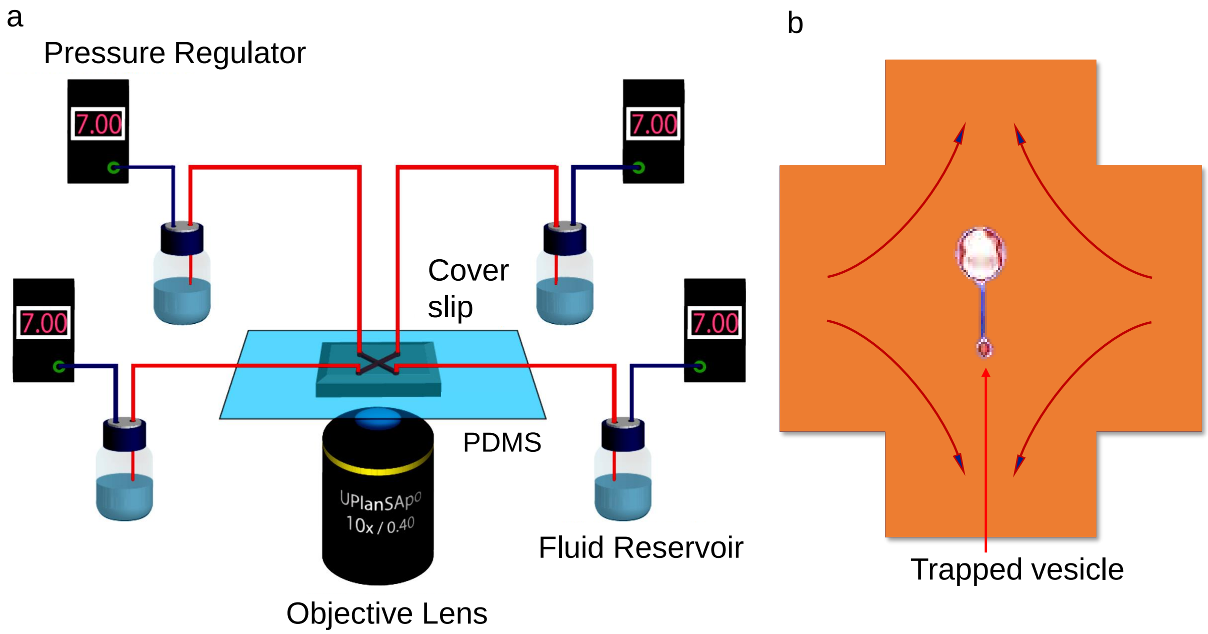


FIG. S1. Experimental set up for vesicle relaxation dynamics in flow. (a) Schematic of the experimental setup used to generate planar extensional flow. Inlet/outlet channels in the microfluidic device are connected to fluidic reservoirs containing vesicle suspension. The fluidic reservoirs are pressurized by regulators controlled by custom LabVIEW program, thereby generating pressure-driven flow in the slot. (b) Schematic of the microfluidic device with a vesicle trapped at stagnation point. The depth of the microfluidic device is 100 $\mu$m.

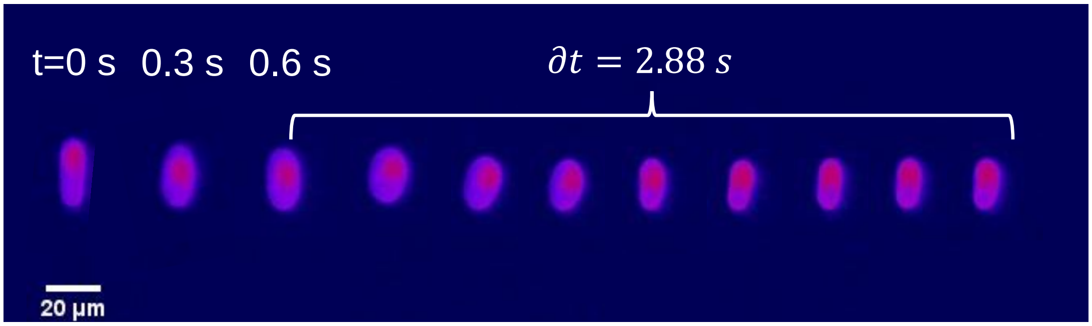


FIG. S2. Time-series of images showing a fluorescently labeled DOPC vesicle with $\nu = 0.95$ relaxing back to an equilibrium shape after being deformed into an ellipsoid shape in extensional flow. The fast phase of relaxation happens in the first $\approx 500$ ms, followed by a slow relaxation.

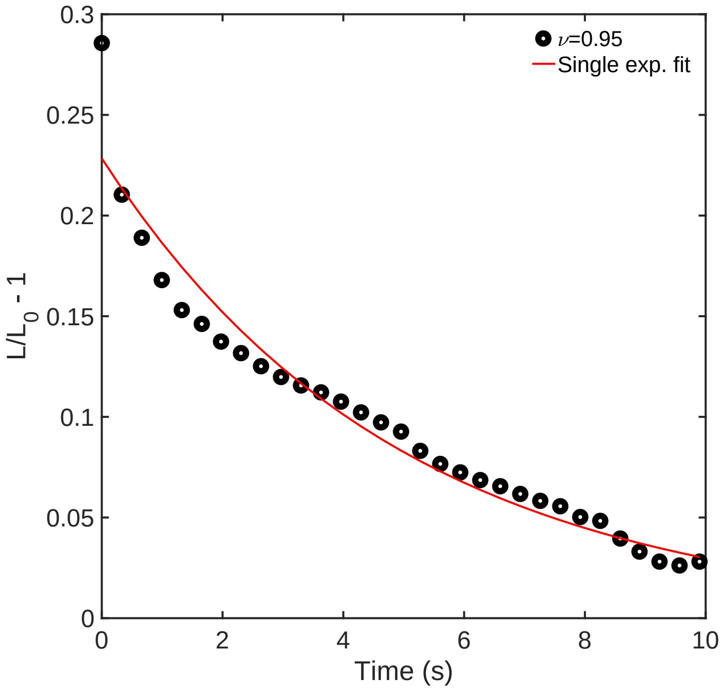


FIG. S3. Relaxation trajectory of a quasi-spherical vesicle with reduced volume $\nu = 0.95$ (black points) with the red curve showing the single mode exponential fit with a relaxation time of $\approx$5 s.

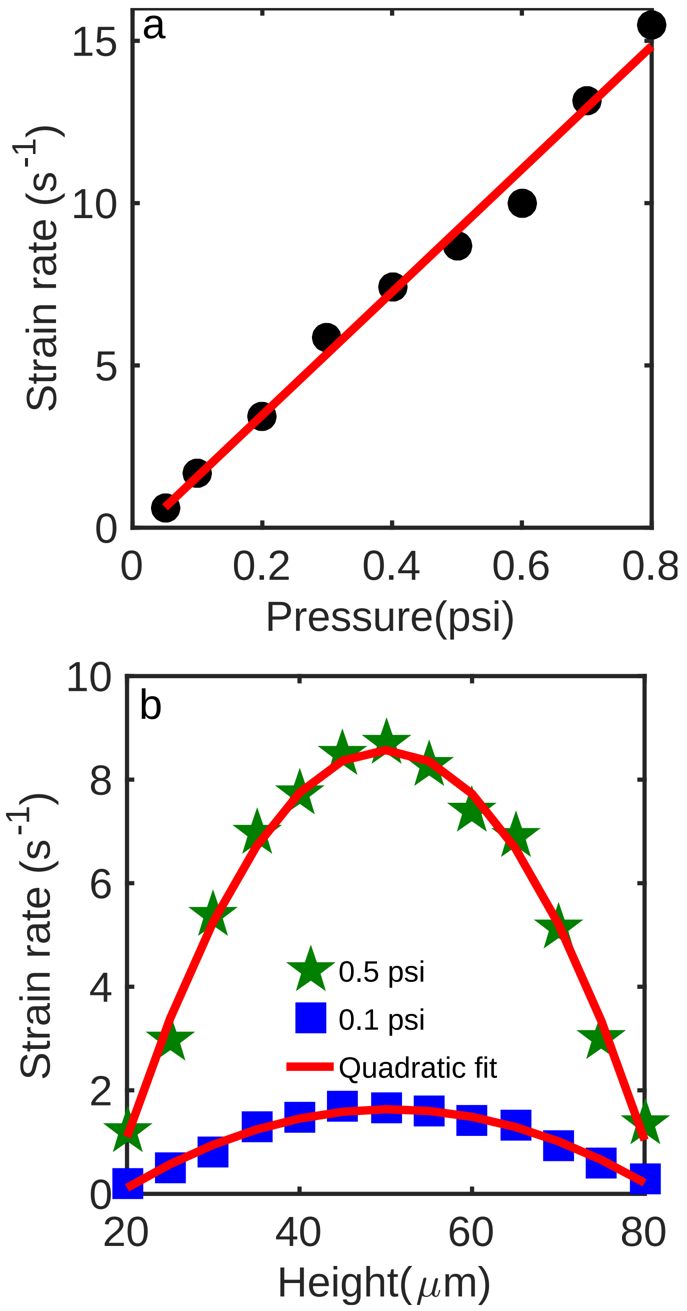


FIG. S4. Flow field characterization in the cross-slot microfluidic device using particle tracking velocimetry (PTV). (a) Strain rate at the center plane of microfluidic device as a function of pressure difference. (b) Strain rates in planar extensional flow as a function of z-position.

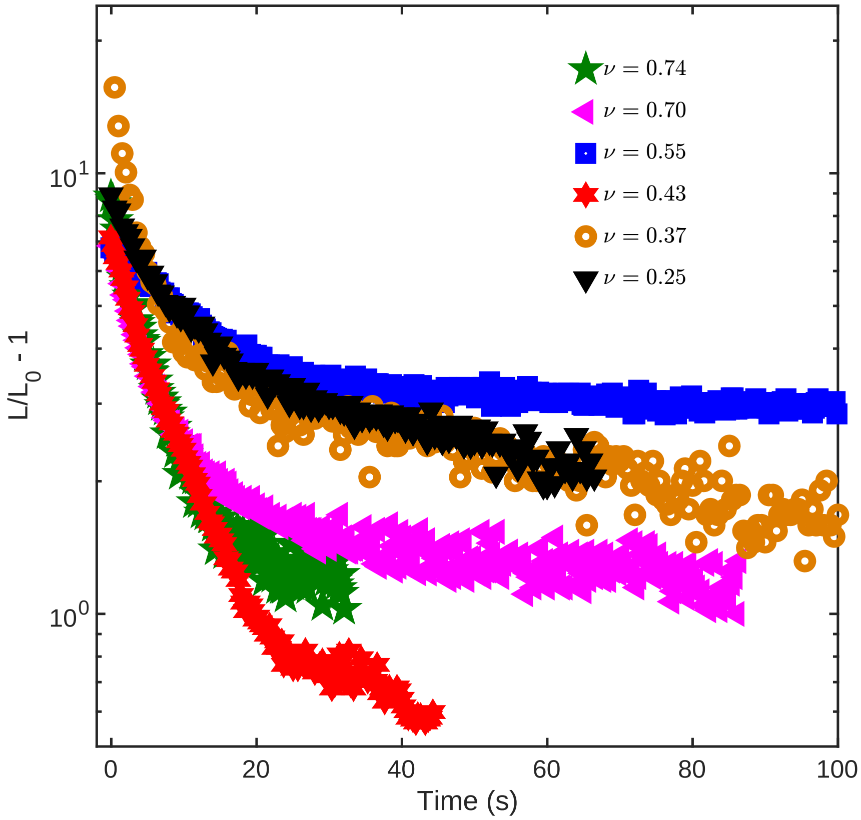


FIG. S5. Semi-log plot of vesicle aspect ratio $L/L_0 - 1$, showing relaxation trajectories of vesicles with different reduced volumes.

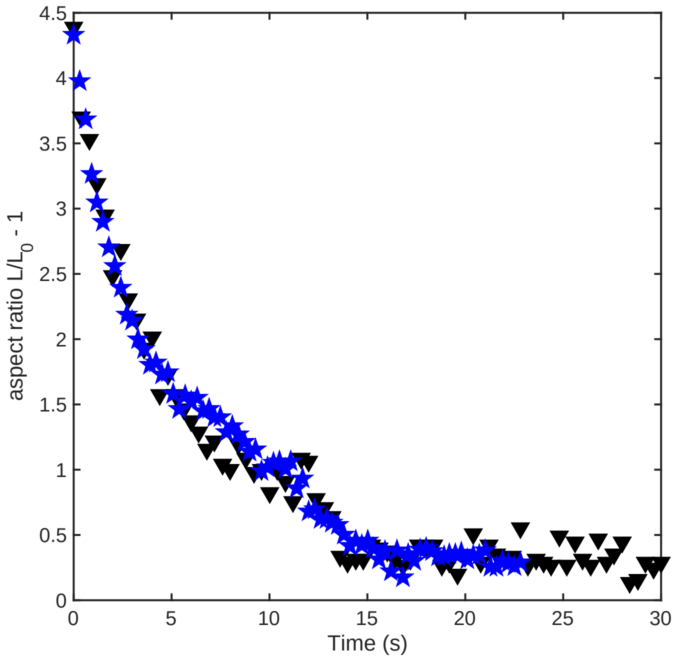


FIG. S6. Relaxation trajectories of a representative vesicle stretched in two successive experiments using the same strain-rate. The relaxation response reveal the nearly deterministic nature of vesicle trajectories.

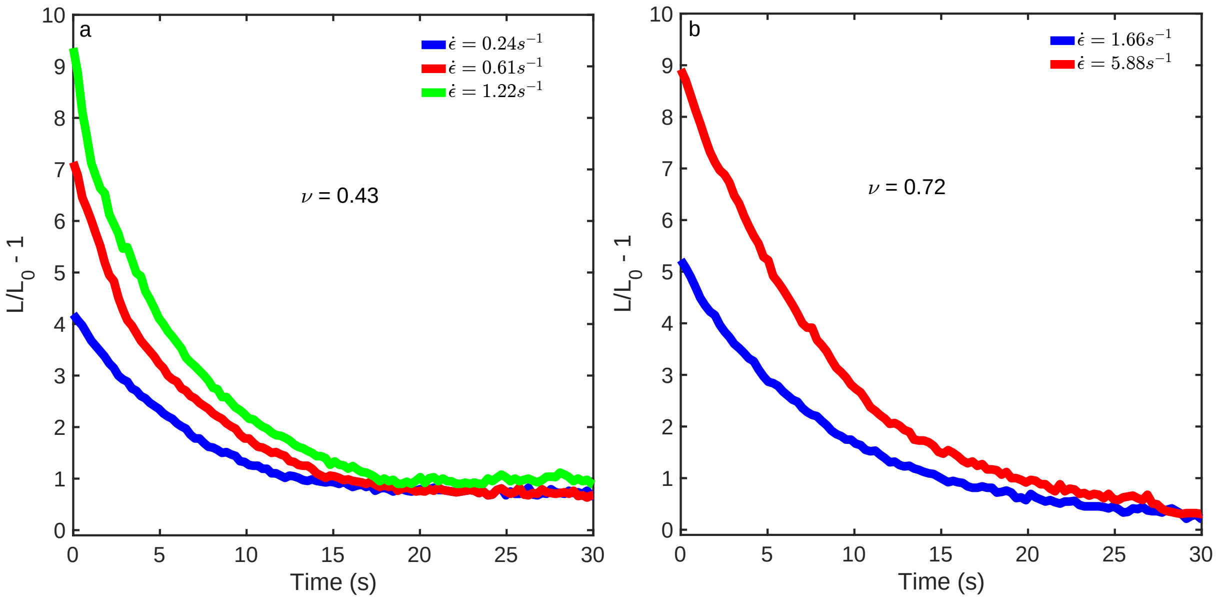


FIG. S7. Repeated relaxation experiments on the same vesicle. (a) Relaxation trajectories of a single vesicle with reduced volume $\nu = 0.43$ stretched multiple times at different strain-rates. (b) Relaxation trajectories of a vesicle with reduced volume $\nu = 0.72$ stretched multiple times at different strain-rates.

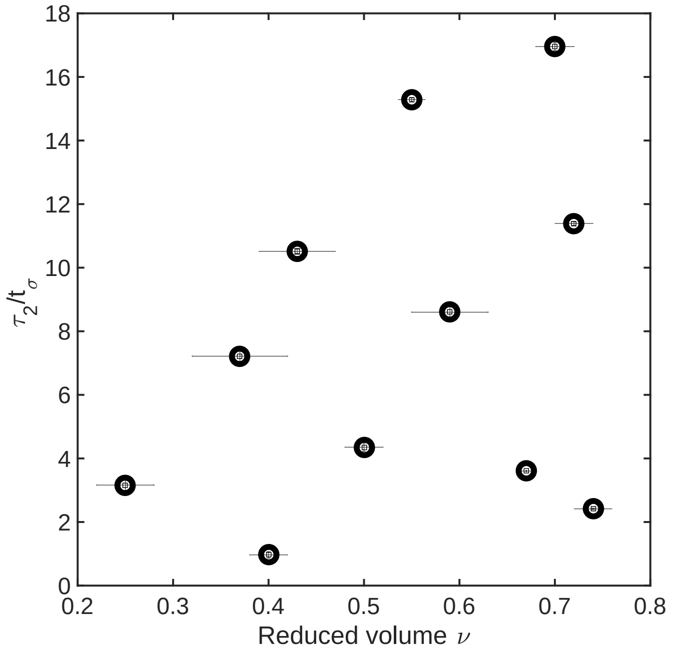


FIG. S8. Normalized slow double-mode relaxation time $\tau_2/t_\sigma$ as a function of reduced volume.

# Supplementary Movies

**Supplementary Movie 1**: A tubular vesicle having reduced volume $\nu = 0.50$ relaxing back from a highly deformed symmetric dumbbell shape. Vesicle is deformed in the bending regime where only thermal fluctuations are flattened out with no area stretching. Movie speed is 2X.

* To whom correspondence must be addressed: cms@illinois.edu

[1] M. Angelova, S. Soléau, P. Méléard, F. Faucon, and P. Bothorel, Preparation of giant vesicles by external ac electric fields. kinetics and applications, in *Trends in Colloid and Interface Science VI* (Springer, 1992) pp. 127–131.
[2] J. B. Dahl, V. Narsimhan, B. Gouveia, S. Kumar, E. S. Shaqfeh, and S. J. Muller, Experimental observation of the asymmetric instability of intermediate-reduced-volume vesicles in extensional flow, Soft matter **12**, 3787 (2016).
[3] R. Dimova, Recent developments in the field of bending rigidity measurements on membranes, Advances in colloid and interface science **208**, 225 (2014).
[4] Y. Xia and G. M. Whitesides, Soft lithography, Annual review of materials science **28**, 153 (1998).
[5] H. Zhou, B. B. Gabilondo, W. Losert, and W. van de Water, Stretching and relaxation of vesicles, Physical Review E **83**, 011905 (2011).
[6] M. Yu, R. B. Lira, K. A. Riske, R. Dimova, and H. Lin, Ellipsoidal relaxation of deformed vesicles, Physical review letters **115**, 128303 (2015).
[7] R. Dimova, U. Seifert, B. Pouligny, S. Förster, and H.-G. Döbereiner, Hyperviscous diblock copolymer vesicles, The European Physical Journal E **7**, 241 (2002).
[8] R. Dasgupta and R. Dimova, Inward and outward membrane tubes pulled from giant vesicles, Journal of Physics D: Applied Physics **47**, 282001 (2014).
[9] J. Pécréaux, H.-G. Döbereiner, J. Prost, J.-F. Joanny, and P. Bassereau, Refined contour analysis of giant unilamellar vesicles, The European Physical Journal E: Soft Matter and Biological Physics **13**, 277 (2004).
[10] D. Kumar, C. M. Richter, and C. M. Schroeder, Conformational dynamics and phase behavior of lipid vesicles in a precisely controlled extensional flow, Soft Matter **16**, 337 (2020).
[11] J.-W. Ha and L. G. Leal, An experimental study of drop deformation and breakup in extensional flow at high capillary number, Physics of fluids **13**, 1568 (2001).
[12] D. R. Bland, *The theory of linear viscoelasticity* (Courier Dover Publications, 2016).
